# Supplementary material for: Pricing Queries Approximately Optimally
Source: arXiv:1508.05347 source file (2015-08-25)
Supplement: Supplementary file 1 [file appendix.tex]

\section{NP-hardness of Optimal Query Pricing}

\begin{theorem}Optimal Pricing of Selection Queries is NP-hard, even when the relation schema
consists of single attribute relations $\{R_1,\ldots,R_t\}$ and bidders are interested either in a unary 
query $R_i$ or in a chain query that involves all relations $R_1,\ldots,R_t$.
\end{theorem}
\begin{proof}
Essentially we show that if buyers are single-minded then computing the optimal
item-pricing is NP-hard. We reduce the SUBSET SUM problem to the optimal pricing problem. 

In subset sum we are given a set of $n$ positive integers $a_1,\ldots,a_n$ and an integer
$B$ and we are asked whether there exists a subset of the integers that sums up to $B$.

Given an instance of Subset Sum we construct the following instance of the optimal pricing problem. 
For each integer $a_j$ we create an item $j$ and two buyers $b_j^1,b_j^2$ interested only in item $j$. 
Buyer $b_j^1$ has value $a_j$ and buyer $b_j^2$ has value $2a_j$.

In addition, there is a buyer $b_*$ who is interested in all items and has a value of $B+A$, where 
$A$ is the total sum of integers $A=\sum_{j=1}^{n}a_j$.

Suppose that the answer to the Subset Sum problem is yes and let $S$ be the set of integers such that
$\sum_{j\in S}a_j=B$. Then the pricing instance admits the following pricing: Price each item 
$j\in S$ with $p_j = 2a_j$ and each item $j\notin S$ with $p_j=a_j$. Now since, $\sum_{j=1}^{n}p_j = B+A$
we know that buyer $b_*$ is also going to buy. The total revenue of this pricing is
$B+A+2A$. The latter $A$ comes from the fact that from each item $j\in S$ we are collecting 
a price of $2a_j$ from bidder $b_j^2$ and for each item $j\notin S$ we are collecting a 
price of $a_j$ from each of $b_j^1,b_j^2$. Thus from the small players we are collecting an extra $2A$ 
of revenue.

Suppose that the answer to the Subset Sum problem is no. Thus there is no subset of items $S$
such that $\sum_{j\in S}a_j=B$. We will now show that there exists no pricing of the items that 
achieves a revenue of $B+3A$. 

Observe that from the small bidders $b_j^1,b_j^2$ of each item $j$ we can collect at most
a price of $2a_j$: let $r_j$ be the revenue collected from the small bidders of item $j$, then
\begin{equation}
r_j = \begin{cases}
p_j & \text{~if~} p_j \in (a_j,2a_j]\\
2p_j & \text{~if~} p_j \in [0,a_j]
\end{cases}
\end{equation}
The above revenue if maximized at either $a_j$ or $2a_j$ and takes maximum value of $2a_j$.

Consider a pricing scheme that serves the big buyer $b_*$. If in that pricing scheme
the price of some item is not $a_j$ or $2a_j$ then, we know that the total 
revenue of such a pricing scheme is smaller than $B+A+2A$, since from the big
buyer we can collect revenue at most $B+A$ and from the small buyers we can
collect at most $2A$ if all items at priced at $a_j$ or $2a_j$ and strictly smaller
if they are assigned some other price. 

Thus the only hope for a pricing scheme to achieve a revenue of $B+3A$ is
if the big buyer $b_*$ is served and all items are charged either $a_j$ or $2a_j$. 

Consider, such a pricing scheme that achieves revenue of $B+3A$. We know that
we are getting revenue of $2A$ from the small buyers, thus we must be getting revenue
of $B+A$ from buyer $b_*$. This means that the total price must be equal to $B+A$. 
Let $S$ be the items in the above charging scheme that are assigned a price of $2a_j$.
Thus for the pricing to achieve revenue of $B+A$ from buyer $b_*$ it must be that:
$\sum_{j\in S}2a_j +\sum_{j\notin S}a_j = B+A \implies \sum_{j\in S} a_j = B$.

However, the latter is a contradiction since we are in the case where the 
answer to the subset sum instance is no.

Thus we showed that the constructed optimal pricing instance has a revenue of 
$B+3A$ if and only if the initial instance of the subset sum problem is 
a yes instance. This completes the proof. 
\end{proof}
